# Supplementary material for: Pixie: A System for Recommending 3+ Billion Items to 200+ Million Users in Real-Time
Source: arXiv:1711.07601 source file (2017-11-21)
Supplement: Supplementary file 1 [file 070appendix.tex]

% !TEX root = paper-pixie.tex

\begin{itemize}
	\item ...
\end{itemize}
